# Supplementary material for: EDGE: Efficient Data Selection for LLM Agents via Guideline Effectiveness
Source: arXiv:2502.12494 source file (2025-02-18)
Supplement: Supplementary file 1 [file 99-appendix.tex]

\section{Appendix}
